# Supplementary material for: Spin-orbit coupling controlled ground state in Sr$_2$ScOsO$_6$
Source: arXiv:1511.07486 source file (2016-04-26)
Supplement: Supplementary file 1 [file supplementary.pdf]

# Supplementary information for:
# Spin-orbit coupling controlled ground state in $Sr_2ScOsO_6$

A. E. Taylor,[1] R. Morrow,[2] R. S. Fishman,[3] S. Calder,[1] A.I. Kolesnikov,[4]
M. D. Lumsden,[1] P. M. Woodward,[2] and A. D. Christianson[1,5]

[1] *Quantum Condensed Matter Division, Oak Ridge National Laboratory, Oak Ridge, Tennessee 37831, USA*
[2] *Department of Chemistry, The Ohio State University, Columbus, Ohio 43210-1185, USA*
[3] *Materials Science and Technology Division, Oak Ridge National Laboratory, Oak Ridge, Tennessee 37831, USA*
[4] *Chemical and Engineering Materials Division, Oak Ridge National Laboratory, Oak Ridge, Tennessee 37831, USA*
[5] *Department of Physics and Astronomy, The University of Tennessee, Knoxville, TN 37996, USA*

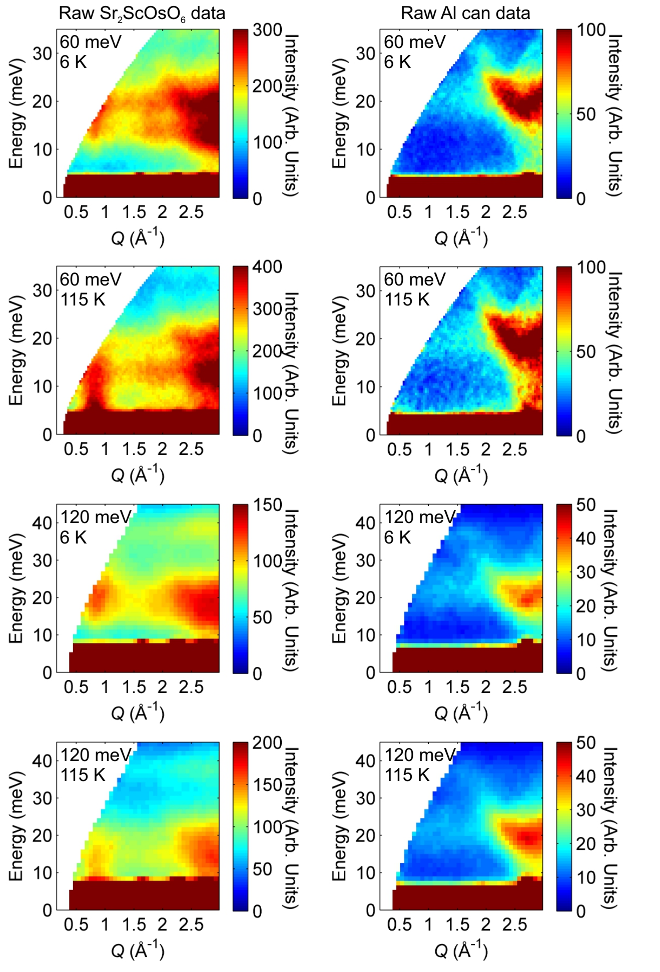


Figure S1. (Color online) Neutron scattering intensity maps showing the $Sr_2ScOsO_6$ data before Al can subtraction and the raw Al can data, as indicated. Labels on each plot indicate the temperature and incident energy used in the measurements.

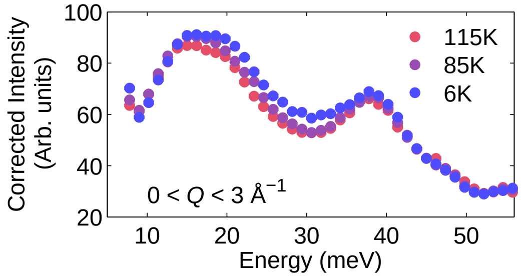


Figure S2. (Color online) Constant wavevector cuts averaged over a large low-Q range, 0 to 3 Å$^{-1}$. Data are from the $E_\mathrm{i} = 120$ meV SEQUOIA datasets measured on $Sr_2ScOsO_6$ with equivalent background measurements of the empty Al can subtracted. Data has been corrected for the Bose thermal population factor.

## INELASTIC NEUTRON SCATTERING

Here we present additional figures from the neutron scattering measurements on SEQUOIA. A closed-cycle refrigerator was used to access temperatures between 6 K and 115 K. Measurements were performed using incident energies,$E_\mathrm{i}$s, of 60 and 120 meV with chopper frequencies of 180 and 300 Hz, respectively. The sample was sealed in a 4 mm-thick flat-plate Al can, and an identical empty can was measured as a background. Empty Al-can measurements were subtracted from all the data sets presented in the main text. Figure S1 shows raw data collected from $Sr_2ScOsO_6$ prior to the empty can subtraction for temperatures above and below $T_\mathrm{N}$. The equivalent raw data used for the empty can background subtraction are also shown, but presented on a lower intensity scale in order that features are visible. It is clear from comparing these intensity maps that the scattering attributed to magnetic fluctuations results from $Sr_2ScOsO_6$, and not a background feature.

In Fig. S2 we present constant wavevector cuts averaged over a large low-Q range, 0 to 3 Å$^{-1}$, in order to include all magnetic scattering and enable us to compare data between different temperatures up to high energies. These data have been corrected for the Bose factor to enable this comparison. The opening of the gap pushes intensity to higher energies in 85 K and 6 K datasets, but the 6 K data appears to converge with the other temperatures at $E \approx 40$ meV, which we identify as $\Gamma$ in the main text. There is a phonon mode present at $E \approx 38$ meV but it's position remains constant with temperature.

The $\chi''(Q, E)$ data presented in Fig. 3(b) was calculated as follows, similar to the method described in

Kermarrec *et al.* [11]. The integrated intensity of the $E_{\mathrm{i}} = 60\,\mathrm{meV}$ data between $5 < E < 9\,\mathrm{meV}$ and $0.5 < Q < 1.2\,\text{Å}^{-1}$ was found at each temperature, then the 6 K data is used as a background. The Bose factor correction is applied to the resulting data, and the highest temperature point is then used to scale the saturated intensity to 1.

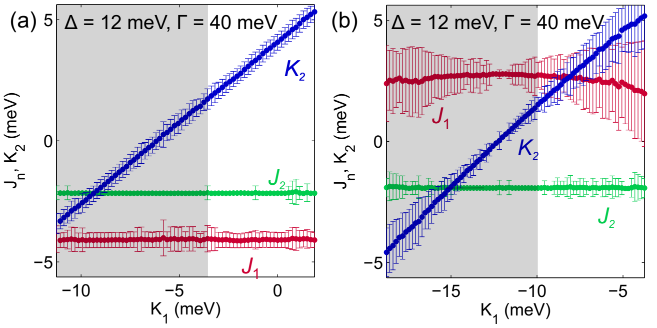


Figure S3. (Color online) Calculated parameters $J_1$, $J_2$, and $K_2$ as a function of $K_1$, showing results for both branches of solutions that met the conditions described in the article. (a) shows results for which $J_1$ is antiferromagnetic, for which both $J_1$ and $J_2$ appear to be stable. Errorbars indicate the spread in each parameter calculated for each $K_1$ starting point, as described in the text.

## SPIN-WAVE MODEL

In addition to the $J_2 \approx 0$ solution discussed in the main article, we attempted to find alternate $J_2 \neq 0$ solutions by searching a large region of parameter space. To include significant NNN interactions we allow both $\mathcal{J}_1$ and $\mathcal{J}_2$ to be anisotropic in spin space. We assume that both exchange interactions are unaffected by the weak monoclinic distortion, so all 6 NNN distances are equivalent. Therefore, the real-space alignment of the spins does not affect the calculation (although the spins are known to lie within the $a$-$b$ plane [23]). As discussed in the article this is justified by the small distortion present in $Sr_2ScOsO_6$. Using the $B$-O-$B'$ angles as a measure of distortion, the most-distorted (i.e. furthest from 180°) angle in $Sr_2ScOsO_6$ is 163.2(3)° at 10 K [23]. Type I order is disrupted in $La_2NaRuO_6$ (which contains $Ru^{5+}$ $4d^3$ ions) giving an incommensurate magnetic ground state, but it has a least-distorted angle of 147.2° [6]. The approximate angle which induces significant changes for $d^3$ ions in DPs is indicated by the crossover from AFM $Sr_2CrSbO_6$ with angles of 166.6(5), 167(6) and 173(4)°, to FM interactions in $Ca_2CrSbO_6$ with angles 153.0(2), 151.9(2) and 152.5(2)° [35] — although the spatial extent of the $3d$ orbitals will have impact on this result.

Therefore, we take the original NN hamiltonian, $\mathcal{H}_{\mathrm{NN}}$, and we add the NNN term, giving

$$\begin{aligned}\mathcal{H} &= \mathcal{H}_{\mathrm{NN}} - \sum_{\mathrm{NNN}} \mathcal{J}_2^{\alpha\beta} S_{i\alpha} S_{j\beta} \\ &= \mathcal{H}_{\mathrm{NN}} - \sum_{\mathrm{NNN}} (J_2 \mathbf{S}_i \cdot \mathbf{S}_j + K_2 S_{ix} S_{jx})\end{aligned}$$

i.e. we have added a $\mathcal{J}_2$ similar to the $\mathcal{J}_1$ term discussed in the article. Explicitly the exchange interactions $\mathcal{J}_1$ and $\mathcal{J}_2$ are written as

$$\begin{aligned}\mathcal{J}_{1\alpha\beta} &= J_1 \delta_{\alpha\beta} + K_1 \delta_{\alpha x} \delta_{\beta x} \\ \mathcal{J}_{2\alpha\beta} &= J_2 \delta_{\alpha\beta} + K_2 \delta_{\alpha x} \delta_{\beta x}\end{aligned}$$

and $\alpha, \beta = \{x, y, z\}$.

To accurately search for solutions in the expanded parameter range, we introduce loose constraints on the parameter space. We solve for the four parameters $J_1$, $J_2$, $K_1$, and $K_2$ based on four conditions as follows. First, the ground state of the Os spins is the type I AFM state depicted in Fig. 1(b) in the main text. To confirm the ground state, we minimize the classical energy, $\epsilon$, among the 64 different spin configurations with distinct Os spins aligned along the $\pm x$ directions in layers $z = 0$, $c/2$, $c$, and $3c/2$. Another stipulation for the local stability of the ground state is that the spin-wave frequencies are real throughout the magnetic Brillouin zone.

The second (third) condition is that the the bottom (top) of the spin-wave band is $\Delta = 12\,\mathrm{meV}$ ($\Gamma = 40\,\mathrm{meV}$). We note that conditions two and three for $\Delta$ and $\Gamma$ are not independent, and that exchange anisotropies $K_1$ and $K_2$ have the same effect on the spin dynamics as a single anisotropy term $\kappa = 3K_2 - 2K_1$. The conditions for the spin-wave energies $\Delta$ and $\Gamma$ are closely satisfied. Finally, we apply a weak constraint using the $T_{\mathrm{N}}$ of 92 K. The expression for the mean-field (MF) transition temperature is $T_{\mathrm{N}} = 2S(S+1)(3(J_2 + K_2) - 2(J_1 + K_1))/3$.

The parameters are calculated over a large range of $K_1$ values. We find ranges of possible solutions for $J_1$, $J_2$ and $K_2$ for each $K_1$, even though $\Delta$ and $\Gamma$ depend only on the combination $\kappa = 3K_2 - 2K_1$, because the problem is under-determined. For different values of $K_1$, we estimate the possible range of the other parameters by their spread for given starting points. This parameter spread occurs because the problem is under-determined, which helps to avoid arriving at a local minimum. Even with $K_1$ fixed, the coupled conditions for the stability of the ground state and for the spin-wave frequencies $\Delta$ and $\Gamma$ are insufficient to completely determine the remaining three parameters. Although $\Delta$ and $\Gamma$ depend only on the combination $\kappa = 3K_2 - 2K_1$, the ranges of solutions in $J_1$ and $J_2$ affect the range in $K_2$ for a fixed $K_1$. For both branches, however, the average value for $\kappa$ is constant over most of the range of $K_1$, as seen in the linear relationship between $K_1$ and $K_2$, Fig. S3. Note that $\epsilon$ does not simply depend on $\kappa$.

We find only two distinct branches of solutions, Fig. S3, one with $J_1 < 0$ (with $J_1 = -4.375\,\mathrm{meV}$, the value determined in the main article, consistent with this result) and

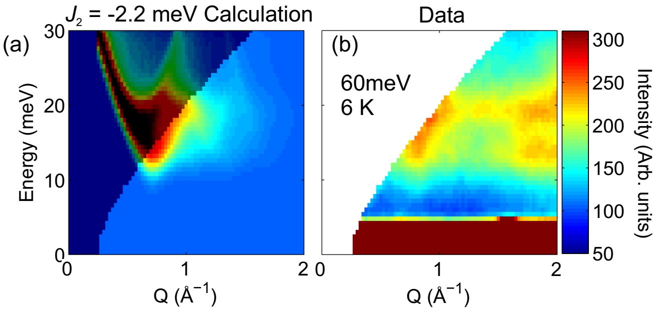


Figure S4. (Color online) Simulated powder-averaged spin-wave spectra for representative finite $J_2$ AFM solution with calculated parameters $K_1 = -3.0$, $J_1 = -4.13$, $J_2 = -2.2$, $K_2 = 2.2\,$meV. This is compared to data collected at $T = 6\,$K on SEQUOIA with $E_{\rm i} = 60\,$meV. The shaded region in the calculations indicates the region of (Q,E) space which is inaccessible in the experimental set-up.

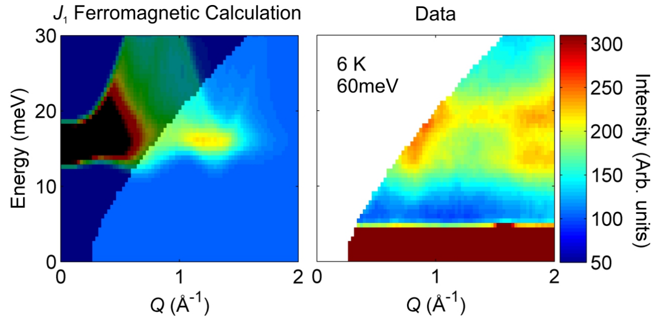


Figure S5. (Color online) Simulated powder-averaged spin-wave spectra for representative $J_1$ ferromagnetic solution with calculated parameters $K_1 = -5.6$, $J_1 = 2.4$, $J_2 = -1.9$, $K_2 = 4.3\,$meV. This is compared to data collected at $T = 6\,$K on SEQUOIA with $E_{\rm i} = 60\,$meV. The shaded region in the calculations indicates the region of (Q,E) space which is inaccessible in the experimental set-up.

the other with $J_1 > 0$. For both branches, the average value for $\kappa$ is constant over the range of $K_1$ (Fig. S3), and the values of $J_1$ and $J_2$ are stable across the solutions. The grey regions show the solutions which are locally stable (have real spin wave solutions) but do not meet the classical condition for stabilizing the type I ground state, $(J_2 + K_2) > 0$ i.e. FM. Having determined the regions of parameter space which match our minimal constraints, we compare the simulated powder-averaged INS cross sections $S(Q, E)$ to the low-temperature data.

Figure S4 shows the results for $J_1$ antiferromagnetic for a representative solution, which qualitatively reproduces the 6 K data very well, similar to the $J_2 = 0$ solution. The results across the full range of $K_1$ are shown in the attached video D12_G40_AFM.mp4. The results with $J_1$ ferromagnetic do not reproduce the observed neutron scattering results, as shown for a representative parameter set in Fig. S5 and additionally over the entire range of parameters in the attached video D12_G40_FM.mp4. The $Os^{5+}$ form factor from Ref. SM[1] was used for all simulations. The observation that solutions with antiferromagnetic $J_1$ provide a better description of the data than ferromagnetic $J_1$ is consistent with expectations considering the relevant NN exchange pathway, see Fig. 1(c). The direct overlap and Os-O-O-Os superexchange interactions are both expected to be AFM, as discussed in the main text.

The simulation presented in Fig. S4 are for parameters $K_1 = -3.0\,$meV, $J_1 = -4.13\,$meV, $J_2 = -2.2\,$meV and $K_2 = 2.2\,$meV. We choose $J_2 = -K_2$ as an interesting case, but the spin wave solutions that result are representative of the range of solutions presented in Fig. S3(a), as seen in the attached video D12_G40_AFM.mp4, because $J_1$ and $J_2$ are stable within the ranges $J_1 = -3.6$ to $-4.7\,$meV and $J_2 = -1.8$ to $2.3\,$meV, and the combination $\kappa = 3K_2 - 2K_1$ is effectively tuning the size of the gap. Consider the particular solution where $J_2 = -K_2$,

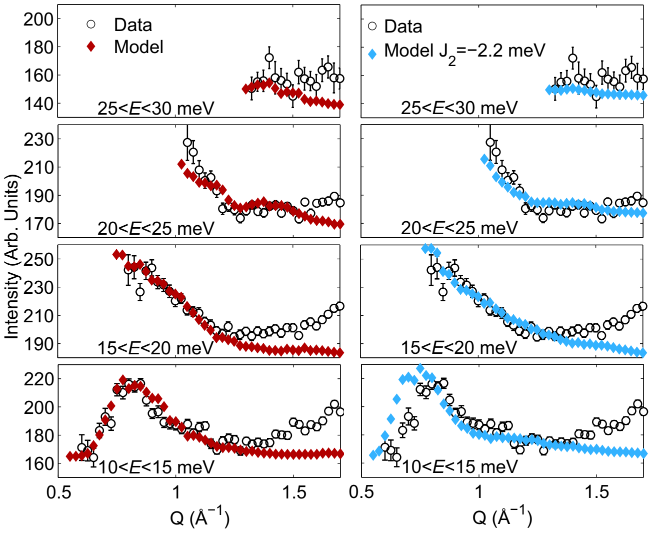


Figure S6. (Color online) Constant-energy cuts through the calculations (diamonds) and data (open circles), for $\mathcal{J}_2 = 0$ model (LHS, red diamonds) and the model with $K_1 = -3.0\,$meV, $J_1 = -4.13\,$meV, $J_2 = -2.2\,$meV and $K_2 = 2.2\,$meV (RHS, blue diamonds). A global scale factor has been used for each calculation, and a flat background applied for each cut.

in this case the term in the Hamiltonian corresponding to the spin direction, $x$, cancels while the $y$ and $z$ components remain finite. This creates a subtle change in the calculated spin-wave specutrum as we will discuss. A range of solutions for $J_2 = -K_2$ are possible, with the exact solution $J_1 = -4.375\,$meV and $K_1 = -3.75\,$meV when $J_2 = -K_2 = 0$ with a mean-field $T_{\rm N} = 181\,$K. The $K_1 = -3.0\,$meV, $J_1 = -4.13\,$meV chosen here result from the mean-field stabilization of the ground state and the $T_{\rm N}$ constraint favoring solutions with slightly lower $T_N = 159\,$K. Both $T_{\rm N}$s are well within the expected range given the frustration in this system.

As the colormaps of the model with $J_2 \approx -2.2$ meV do not distinguish it from a model with $J_2 \approx 0$, we present constant-energy cuts through the data and each model in Fig. S6. The comparison shows that the non-zero $y$ and $z$ components in the Hamiltonian, $\mathcal{J}_{2yy} = \mathcal{J}_{2zz} \neq 0$, appear to have greatest influence on the spinwave spectrum at low energy, and here in the 10<E<15 meV cut it is apparent that the $J_2 = 0$ model provides a much better description of the data. This is also a physically reasonably model in terms of relevant exchange pathways, as discussed in the main text.

As a check to the validity of our results, we also tried our calculations for different values of $\Gamma$ and $\Delta$. Here we show the calculated exchange parameters for $\Delta = 12$ meV and $\Gamma = 35$ meV, Fig. S7(a) and (b), and $\Delta = 8$ meV and $\Gamma = 40$ meV, Fig. S7(c) and (d). The resulting $S(Q, E)$ from all of these cases as shown in videos D12_G35_AFM.mp4, D12_G35_FM.mp4, D8_G40_AFM.mp4 and D8_G40_FM.mp4, and none of the parameters reproduce the data like the $\Delta = 12$ meV and $\Gamma = 40$ meV results.

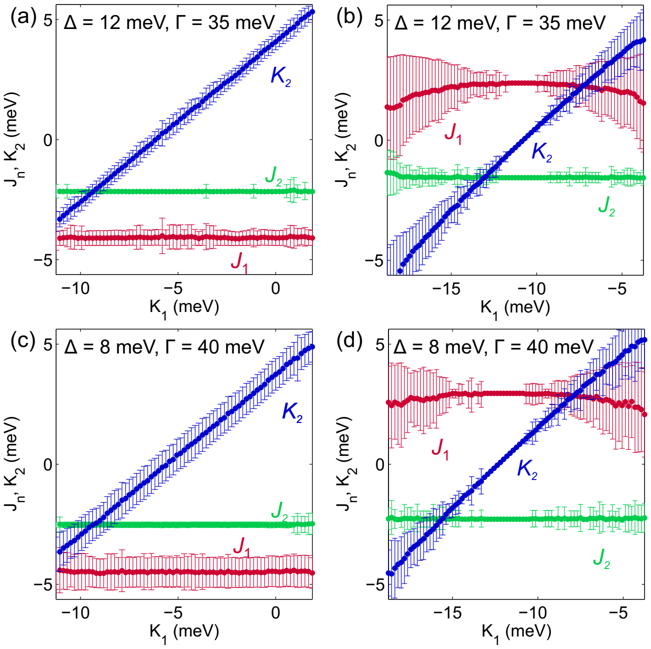


Figure S7. (Color online) Calculated parameters $J_1$, $J_2$, and $K_2$ as a function of $K_1$, for alternative values of $\Gamma$ ((a) and (b)) and $\Delta$ ((c) and (d)) showing results for both branches of solutions. Again the errorbars indicate the spread in each parameter calculated for each $K_1$ starting point, as described in the text.


[1] K. Kobayashi, T. Nagao, and M. Ito, Acta Crystallographica Section A Foundations of Crystallography **67**, 473 (2011).
